# Supplementary material for: Isotope Shifts of Radium Monofluoride Molecules
Source: arXiv:2105.10549 source file (2021-05-21)
Supplement: Supplementary file 1 [file Isotope_Shifts_of_Radium_Monofluoride_Molecules_Supplemental_Material.pdf]

# Isotope Shifts of Radium Monofluoride Molecules


S.M. Udrescu,[1,*] A.J. Brinson,[1] R.F. Garcia Ruiz,[1,2,†] K. Gaul,[3] R. Berger,[3,‡] J. Billowes,[4] C.L. Binnersley,[4] M.L. Bissell,[4] A.A. Breier,[5] K. Chrysalidis,[2] T.E. Cocolios,[6] B.S. Cooper,[4] K.T. Flanagan,[4,7] T.F. Giesen,[5] R.P. de Groote,[8] S. Franchoo,[9] F.P. Gustafsson,[6] T.A. Isaev,[10] Á. Koszorús,[6] G. Neyens,[2,6] H.A. Perrett,[4] C.M. Ricketts,[4] S. Rothe,[2] A.R. Vernon,[4] K.D.A. Wendt,[11] F. Wienholtz,[2,12] S.G. Wilkins,[2] and X.F. Yang[13]

[1] *Massachusetts Institute of Technology, Cambridge, MA 02139, USA*
[2] *CERN, CH − 1211 Geneva 23, Switzerland*
[3] *Fachbereich Chemie, Philipps − Universität Marburg, Hans − Meerwein − Straße 4, 35032 Marburg, Germany*
[4] *School of Physics and Astronomy, The University of Manchester, Manchester M13 9PL, United Kingdom*
[5] *Laboratory for Astrophysics, Institute of Physics, University of Kassel, 34132 Kassel, Germany*
[6] *KU Leuven, Instituut voor Kern − en Stralingsfysica, B − 3001 Leuven, Belgium*
[7] *Photon Science Institute, The University of Manchester, Manchester M13 9PY, United Kingdom*
[8] *Department of Physics, University of Jyväskylä, Survontie 9, Jyväskylä, FI − 40014, Finland*
[9] *Institut de Physique Nucleaire d'Orsay, F − 91406 Orsay, France*
[10] *NRC Kurchatov Institute-PNPI, Gatchina, Leningrad district 188300, Russia*
[11] *Institut für Physik, Johannes Gutenberg − Universität Mainz, D − 55128 Mainz, Germany*
[12] *Institut für Physik, Universität Greifswald, D − 17487 Greifswald, Germany*
[13] *School of Physics and State Key Laboratory of Nuclear Physics and Technology, Peking University, Beijing 100971, China*



(Dated: December 4, 2020)


## THEORETICAL METHODS

Transition energies for different isotopologues of RaF were calculated at the level of relativistic Fock-Space Coupled Cluster including Singles and Doubles amplitudes (FSCCSD). These calculations were carried out with the program package DIRAC19 [1]. The nuclear charge density of nucleus $A$ was described by a normalized Gaussian function $\rho_A(\vec{r}_i) = \rho_0 \mathrm{e}^{-\zeta|\vec{r}_i - \vec{r}_A|^2}$ with $\zeta = \frac{3}{2\langle r^2 \rangle}$ being characterized by an empirically determined root-mean-square nuclear radius of $\langle r^2 \rangle^{1/2} = \left[0.836 A^{1/3} + 0.570\right]$ fm [2], instead of a homogeneously charged solid sphere as was assumed as a starting point in previous atomic calculations used to determine the experimental nuclear charge radii in Radium isotopes [3, 4]. Here $\vec{r}_i$ and $\vec{r}_A$ denote the position vector of electron $i$ and nucleus $A$, respectively. Calculations were carried out for different root-mean-square nuclear radii that within this model correspond to isotopologues of $^{A}\mathrm{Ra}^{19}\mathrm{F}$, with even values for the Ra nucleus mass, $A$, ranging from $A = 212$ up to $A = 232$, in addition to the isotopologues with $A = 213, 223, 225$.

Calculations were performed using the s,p,d,f-subset of the ANO-RCC basis on Ra and the s,p,d-subset of the ANO-RCC basis on F. In these calculations, the 6s, 6p and 7s shells of Ra and the 2s and 2p shells of F are correlated (17 electrons) and are therefore denoted as FSCCSD(17e). All calculations were repeated for bond lengths of $r_{\mathrm{RaF}} = 4.0$, 4.1, 4.2, 4.25, 4.3 and 4.4 $a_0$, which covers the region around the equilibrium structure of the electronic ground state. For each bond length, the isotope shift constant $F(r_{\mathrm{RaF}}) = \frac{\partial \delta \tilde{\nu}}{\partial \delta \langle r^2 \rangle}(r_{\mathrm{RaF}})$ is determined by a linear fit of the total energy of RaF for different electronic states in dependence of the Ra mass (see Fig. 1).

TABLE I. Isotope shift constants $F = \frac{\partial \delta \tilde{\nu}}{\partial \delta \langle r^2 \rangle}$ of electronic states in RaF for different bond lengths at the FSCCSD(17e) level. FSCCSD(27e) calculations are shown in square brackets for a bond length of $r_{\mathrm{RaF}} = 4.3\, a_0$. Isotope shift constants $F$ of the $A^2\Pi_{1/2} \leftarrow X^2\Sigma_{1/2}$ transition correspond to the slopes in Fig. 1. For all calculated isotope shifts fit errors are $< 10^{-3}\ \frac{\mathrm{cm}^{-1}}{\mathrm{fm}^2}$.

| $r_{\mathrm{RaF}}$ $(a_0)$ | $F$ $\left(\frac{\mathrm{cm}^{-1}}{\mathrm{fm}^2}\right)$ | | |
|---|---|---|---|
| | $X^2\Sigma_{1/2}$ | $A^2\Pi_{1/2}$ | $A^2\Pi_{1/2} \leftarrow X^2\Sigma_{1/2}$ |
| 4.0 | 0.756 | −0.015 | −0.771 |
| 4.1 | 0.758 | −0.021 | −0.778 |
| 4.2 | 0.760 | −0.027 | −0.787 |
| 4.25 | 0.762 | −0.030 | −0.792 |
| 4.3 | 0.764 | −0.033 | −0.797 [−0.825] |
| 4.4 | 0.769 | −0.039 | −0.808 |

In order to estimate the quality of this method, FSCSSD calculations with an extended basis set of 33 s, 29 p, 20 d, 14 f, 7 g, and 6 h functions for Ra and additionally correlating the 5d shell of Ra (27 correlated electrons) (FSCCSD(27e)) were carried out for the isotopologues $^{224}\mathrm{Ra}^{19}\mathrm{F}$, $^{226}\mathrm{Ra}^{19}\mathrm{F}$ and $^{228}\mathrm{Ra}^{19}\mathrm{F}$ at a bond length of 4.3 $a_0$. The resulting isotope shifts constants for different bond lengths of RaF are shown in Table I.

The same basis set that was employed in the FSCCSD(27e) calculations was used in an atomic FSCCSD calculation of $\mathrm{Ra}^+$, in which 19 electrons (5d, 6s, 6p and 7s shells) were correlated. These atomic calculations were used to allow a direct comparison between our measurements and previous isotope shift measure-

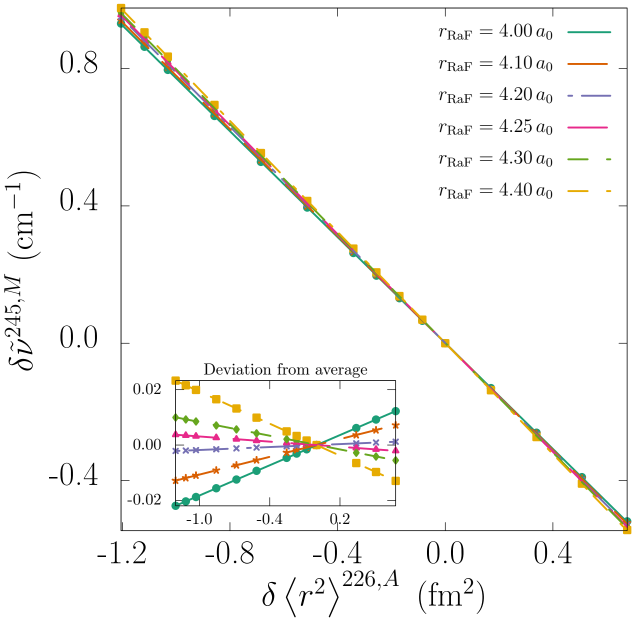


FIG. 1. Isotope shifts as a function of the changes in the charge radius with respect to the reference charge radius that corresponds within the applied model to the isotopologue $^{226}$Ra$^{19}$F molecule calculated at the level of FSCCSD(17e). Each color corresponds to one of the six different bond lengths. In the inset (bottom left), the deviation from the average over all bond lengths is shown for each bond length. The slopes of the linear fits for each bond length are given in Table I.

ments in the radium ion. In the present work, the nucleus is modeled as a Gaussian distribution. In all FSCCSD calculations, the active space was restricted to virtual orbitals below 1000 $E_{\rm h}$.

Vibrational corrections to isotope shift constants were calculated from a fourth-degree polynomial fit of the bond length dependence of isotope shifts:

$$F(r_{\rm RaF}) \approx \sum_{k=0} c_k r_{\rm RaF}^k \,. \qquad (1)$$

Vibrational wave functions were received in a one-dimensional discrete variable representation (DVR) scheme [5] employing the potentials of the electronic ground and excited states calculated in Ref. [6] using the the reference isotopologue $^{226}$Ra$^{19}$F. The dependence of the vibrational wave functions on different masses of Ra was determined to be $\ll 1\,\%$. A sketch of the electronic potentials of the $X^2\Sigma^+$ and $A^2\Pi_{1/2}$ from Ref. [6] are shown in Fig. 2. The linear moments in the figure are shown for the first four vibrational levels to illustrate for which bond lengths the vibronic expectation values are evaluated. The bond length dependence of the isotope shift of the $X^2\Sigma^+$ and $A^2\Pi_{1/2}$ states is given relative to that of the 0th vibrational level. The vibronic expectation value is calculated as

$$F = \langle v|F(r_{\rm RaF})|v\rangle = \sum_{k=0} \langle v|r_{\rm RaF}^k|v\rangle c_k \,, \qquad (2)$$

with $c_k$ being coefficients of the fourth-order polynomial fit of the bond length dependence of isotope shifts. The crossing points of $\langle \frac{\partial\delta\tilde{\nu}}{\partial\delta\langle r^2\rangle}\rangle$ (points and stars) with the linear moments (gray vertical lines) give the leading-order contribution to the vibronic expectation values. For the $A^2\Pi_{1/2}$ state this is almost identical to the full expectation values (orange dotted/dashed lines), whereas for the $X^2\Sigma^+$ state non-linear contributions are much more important.

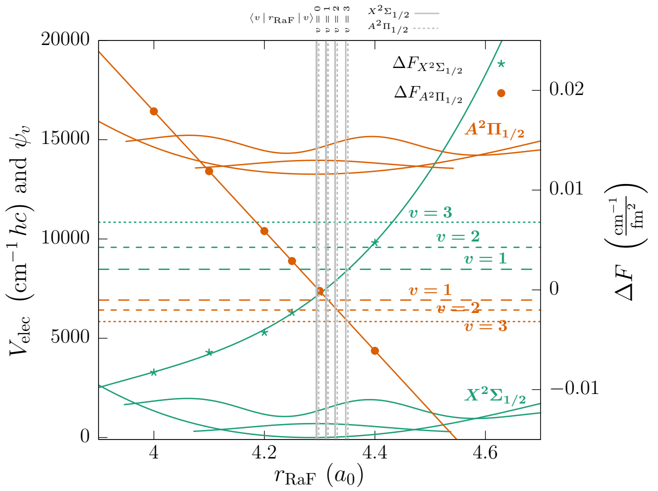


FIG. 2. Electronic potentials of the $X^2\Sigma^+$ and $A^2\Pi_{1/2}$ states. The vibrational wave functions are shown for the zeroth and third vibrational states, respectively. Wave functions are shifted to the energy of the vibrational level and scaled arbitrarily for better representation (see text for more details). Isotope shift constants are shown relative to the vibrational ground state ($\Delta F = (F - \langle v=0|F(r_{\rm RaF})|v=0\rangle)$) for both electronic states as function of $r_{\rm RaF}$ (dots and stars) alongside polynomial approximations and vibronic expectation values (horizontal dotted lines).

## ISOTOPE SHIFT DERIVATION

In the Dunham model [7], the rovibrational energy levels of a diatomic molecule are given by

$$E_{\nu,J} = \sum_{k,l\geq 0} Y_{kl}\left(\nu+\frac{1}{2}\right)^k [J(J+1)]^l, \qquad (3)$$

where $\nu$ and $J$ are the vibrational and rotational quantum numbers, respectively, for a given electronic level, and $Y_{kl}$ are the Dunham coefficients in units of frequency.

It can be shown [8, 9] that these coefficients have an explicit dependence on the reduced mass of the molecule expressed as

$$Y_{kl} = \mu^{-(k/2+l)} U_{kl}. \tag{4}$$

Ross et al. [10] showed that further isotope-dependent corrections are needed for the expression above, to account for the breakdown of the Born-Oppenheimer approximation and the Jeffreys-Wentzel-Brillouin-Kramers (JWBK) approximation [11–14] used in the Dunham model derivation [15–17]. The size of the nuclei of the atoms in the molecule produces a further shift of the energy levels [8, 9, 18, 19], introducing a field shift correction. The modified expression is given by

$$\begin{aligned} Y_{kl} = \mu^{-(k/2+l)} U_{kl} \Bigg[ 1 + m_\mathrm{e} \left( \frac{\Delta^A_{kl}}{M_A} + \frac{\Delta^B_{kl}}{M_B} \right) \\ + V^A_{kl} \langle r^2 \rangle_A + V^B_{kl} \langle r^2 \rangle_B \Bigg], \end{aligned} \tag{5}$$

where $M_A$ and $M_B$ are the masses of the two atoms in the molecule, while $\Delta^\alpha_{kl}$ and $\Delta^B_{kl}$ are mass-independent corrections for each of the two atoms. $\langle r^2 \rangle_A$ and $\langle r^2 \rangle_B$ are the nuclear mean-squared charge radii of the two nuclei in the molecule, while $V^A_{kl}$ and $V^B_{kl}$ quantify the magnitude of the change of a given Dunham parameter due to the nuclear size. These parameters can be related to the electron density at the given nucleus, as well as the first and second derivative of this density with respect to internuclear axis (see [9] for a more detailed discussion).

In our case, given that we are interested in variations between molecules in which only the radium nucleus is changed, the fluorine nucleus contributions can be neglected ($\mathcal{O}(M_\mathrm{F}, \langle r^2 \rangle_\mathrm{F})$). Eq. 5 reduces to:

$$\begin{aligned} Y_{kl} = \mu^{-(k/2+l)}_\mathrm{RaF} U_{kl} \left[ 1 + m_\mathrm{e} \frac{\Delta^\mathrm{Ra}_{kl}}{M_\mathrm{Ra}} + V^\mathrm{Ra}_{kl} \langle r^2 \rangle_\mathrm{Ra} \right] \\ + \mathcal{O}(M_\mathrm{F}, \langle r^2 \rangle_\mathrm{F}). \end{aligned} \tag{6}$$

In this approach, the parameter $U_{kl}$ is independent of mass or volume effects, being the same for all isotopes. At the energy resolution of our experiment, we are mainly sensitive to changes in the electronic energy $E_\mathrm{el}$, associated to $Y_{00}$ and the first-order vibrational energy $E_\mathrm{vib}$, linked to $Y_{10}$. So that the transition energy $E$ is given by

$$E = \overbrace{Y'_{00} - Y''_{00}}^{E_\mathrm{el}} + \overbrace{Y'_{10} - Y''_{10}}^{E_\mathrm{vib}}. \tag{7}$$

Thus, the energy of the electronic transition between the $X^2\Sigma^+$ and $A^2\Pi_{1/2}$ state for a given RaF isotopologue, $\alpha$, is given by

$$\begin{aligned} E^{\alpha,\Pi,\Sigma}_\mathrm{el} &= Y^{\alpha,\Pi}_{00} - Y^{\alpha,\Sigma}_{00} \\ &= U^\Pi_{00} \left[ 1 + m_\mathrm{e} \frac{\Delta^{\alpha,\Pi}_{00}}{M_\alpha} + V^{\alpha,\Pi}_{00} \langle r^2 \rangle_\alpha \right] \\ &\quad - U^\Sigma_{00} \left[ 1 + m_\mathrm{e} \frac{\Delta^{\alpha,\Sigma}_{00}}{M_\alpha} + V^{\alpha,\Sigma}_{00} \langle r^2 \rangle_\alpha \right] \\ &= U^\Pi_{00} - U^\Sigma_{00} + \frac{m_\mathrm{e}}{M_\alpha} (\Delta^{\alpha,\Pi}_{00} U^\Pi_{00} - \Delta^{\alpha,\Sigma}_{00} U^\Sigma_{00}) \\ &\quad + (V^{\alpha,\Pi}_{00} U^\Pi_{00} - V^{\alpha,\Sigma}_{00} U^\Sigma_{00}) \langle r^2 \rangle_\alpha. \end{aligned} \tag{8}$$

This expression can be re-written as

$$E^{\alpha,\Pi,\Sigma}_\mathrm{el} = U^\Pi_{00} - U^\Sigma_{00} + \frac{\Delta(\Delta^{\alpha,\Pi-\Sigma}_{00})}{M_\alpha} + \Delta V^{\alpha,\Pi-\Sigma}_{00} \langle r^2 \rangle_\alpha, \tag{9}$$

with

$$\Delta(\Delta^{\alpha,\Pi-\Sigma}_{00}) \equiv m_\mathrm{e} (\Delta^{\alpha,\Pi}_{00} U^\Pi_{00} - \Delta^{\alpha,\Sigma}_{00} U^\Sigma_{00}), \tag{10}$$

and

$$\Delta V_{00} \equiv V^{\alpha,\Pi}_{00} U^\Pi_{00} - V^{\alpha,\Sigma}_{00} U^\Sigma_{00}. \tag{11}$$

The equivalent formula for the vibrational energy $E_\mathrm{vib}$, for the same vibrational excitation, $\nu$, of the $X^2\Sigma^+$ and $A^2\Pi_{1/2}$ electronic levels is given by

$$\begin{aligned} &E^{\alpha,\Pi,\Sigma,\nu}_\mathrm{vib} \\ &= (Y^{\alpha,\Pi}_{10} - Y^{\alpha,\Sigma}_{10})(\nu + 1/2) \\ &= \mu^{-1/2}_\alpha U^\Pi_{10} \left[ 1 + m_\mathrm{e} \frac{\Delta^{\alpha,\Pi}_{10}}{M_\alpha} + V^{\alpha,\Pi}_{10} \langle r^2 \rangle_\alpha \right] (\nu + 1/2) \\ &- \mu^{-1/2}_\alpha U^\Sigma_{10} \left[ 1 + m_\mathrm{e} \frac{\Delta^{\alpha,\Sigma}_{10}}{M_\alpha} + V^{\alpha,\Sigma}_{10} \langle r^2 \rangle_\alpha \right] (\nu + 1/2), \end{aligned} \tag{12}$$

and

$$\begin{aligned} E^{\alpha,\Pi,\Sigma,\nu}_\mathrm{vib} &= \mu^{-1/2}_\alpha (U^\Pi_{10} - U^\Sigma_{10})(\nu + 1/2) \\ &\quad + \mu^{-1/2}_\alpha \frac{m_\mathrm{e}}{M_\alpha} (\Delta^{\alpha,\Pi}_{10} U^\Pi_{10} - \Delta^{\alpha,\Sigma}_{10} U^\Sigma_{10})(\nu + 1/2) \\ &\quad + \mu^{-1/2}_\alpha (V^{\alpha,\Pi}_{10} U^\Pi_{10} - V^{\alpha,\Sigma}_{10} U^\Sigma_{10})(\nu + 1/2) \langle r^2 \rangle_\alpha. \end{aligned} \tag{13}$$

Similarly, it can be expressed as

$$\begin{aligned} E^{\alpha,\Pi,\Sigma,\nu}_\mathrm{vib} &= \mu^{-1/2}_\alpha (U^\Pi_{10} - U^\Sigma_{10})(\nu + 1/2) \\ &+ \mu^{-1/2}_\alpha \frac{\Delta(\Delta^{\alpha,\Pi-\Sigma}_{10})}{M_\alpha} (\nu + 1/2) + \mu^{-1/2}_\alpha \Delta V^{\alpha,\Pi-\Sigma}_{10} (\nu + 1/2) \langle r^2 \rangle_\alpha, \end{aligned} \tag{14}$$

where

$$\Delta(\Delta^{\alpha,\Pi-\Sigma}_{10}) \equiv m_\mathrm{e} (\Delta^{\alpha,\Pi}_{10} U^\Pi_{10} - \Delta^{\alpha,\Sigma}_{10} U^\Sigma_{10}), \tag{15}$$

and

$$\Delta V_{10} \equiv V_{10}^{\alpha,\Pi} U_{10}^{\Pi} - V_{10}^{\alpha,\Sigma} U_{10}^{\Sigma}. \tag{16}$$

Using Eq. 9, the isotope shift between two isotopologues $\alpha$ and $\alpha'$ associated to the electronic energy between the $\Pi$ and $\Sigma$ state is given by

$$\begin{aligned} E_{\mathrm{el}}^{\alpha',\Pi,\Sigma} - E_{\mathrm{el}}^{\alpha,\Pi,\Sigma} &= \Delta(\Delta_{00}^{\alpha,\Pi-\Sigma}) \left( \frac{1}{M_{\alpha'}} - \frac{1}{M_\alpha} \right) \\ &\quad + \Delta V_{00}^{\alpha,\Pi-\Sigma} (\langle r^2 \rangle_{\alpha'} - \langle r^2 \rangle_{\alpha}) \\ &= \Delta(\Delta_{00}^{\alpha,\Pi-\Sigma}) \left( \frac{M_\alpha - M_{\alpha'}}{M_\alpha M_{\alpha'}} \right) \\ &\quad + \Delta V_{00}^{\alpha,\Pi-\Sigma} \delta \langle r^2 \rangle_{\alpha\alpha'} \end{aligned} \tag{17}$$

Similarly, Eq. 14 gives the isotope shift associated with the vibrational energy

$$\begin{aligned} & E_{\mathrm{vib}}^{\alpha',\Pi,\Sigma,\nu} - E_{\mathrm{vib}}^{\alpha,\Pi,\Sigma,\nu} \\ & = \Delta(\Delta_{10}^{\alpha,\Pi-\Sigma}) \left( \frac{M_\alpha {\mu'_\alpha}^{-1/2} - M_{\alpha'} \mu_\alpha^{-1/2}}{M_\alpha M_{\alpha'}} \right) (\nu + 1/2) \\ & + \Delta V_{10}^{\alpha,\Pi-\Sigma} \left( \frac{\langle r^2 \rangle_{\alpha'}}{\sqrt{\mu_{\alpha'}}} - \frac{\langle r^2 \rangle_{\alpha}}{\sqrt{\mu_\alpha}} \right) (\nu + 1/2). \end{aligned} \tag{18}$$

Therefore, the overall energy shift due to electronic and vibrational energy is given by

$$\begin{aligned} & \Delta E^{\alpha,\alpha',\Pi,\Sigma,\nu} \\ & = E_{\mathrm{el}}^{\alpha',\Pi,\Sigma} - E_{\mathrm{el}}^{\alpha,\Pi,\Sigma} + E_{\mathrm{vib}}^{\alpha',\Pi,\Sigma,\nu} - E_{\mathrm{vib}}^{\alpha,\Pi,\Sigma,\nu} \\ & = \Delta(\Delta_{00}^{\alpha,\Pi-\Sigma}) \left( \frac{M_\alpha - M_{\alpha'}}{M_\alpha M_{\alpha'}} \right) + \Delta V_{00}^{\alpha,\Pi-\Sigma} \delta \langle r^2 \rangle_{\alpha\alpha'} \\ & + \Delta(\Delta_{10}^{\alpha,\Pi-\Sigma}) \left( \frac{M_\alpha \mu_{\alpha'}^{-1/2} - M_{\alpha'} \mu_\alpha^{-1/2}}{M_\alpha M_{\alpha'}} \right) (\nu + 1/2) \\ & + \Delta V_{10}^{\alpha,\Pi-\Sigma} \left( \frac{\langle r^2 \rangle_{\alpha'}}{\sqrt{\mu_{\alpha'}}} - \frac{\langle r^2 \rangle_{\alpha}}{\sqrt{\mu_\alpha}} \right) (\nu + 1/2) \\ & \approx \Delta V_{00}^{\alpha,\Pi-\Sigma} \delta \langle r^2 \rangle_{\alpha\alpha'} + \Delta V_{10}^{\alpha,\Pi-\Sigma} \left( \frac{\langle r^2 \rangle_{\alpha'}}{\sqrt{\mu_{\alpha'}}} - \frac{\langle r^2 \rangle_{\alpha}}{\sqrt{\mu_\alpha}} \right) (\nu + 1/2). \end{aligned} \tag{19}$$

The terms containing $\Delta(\Delta_{00}^{\alpha,\Pi-\Sigma})$ and $\Delta(\Delta_{10}^{\alpha,\Pi-\Sigma})$ are expected to be less than 0.001 $\mathrm{cm}^{-1}$ in magnitude, based on mass shift values from $Ra^+$ [3], and the $\widetilde{\omega}_e$ values of the $A^2\Pi_{1/2}$ and $X^2\Sigma^+$ states in $^{226}Ra^{19}F$ [20]. Hence they are neglected in the present study. When the term $\frac{\delta \langle r^2 \rangle_{\alpha\alpha'}}{\sqrt{\mu_\alpha}}$ is used instead of $\left( \frac{\langle r^2 \rangle_{\alpha'}}{\sqrt{\mu_{\alpha'}}} - \frac{\langle r^2 \rangle_{\alpha}}{\sqrt{\mu_\alpha}} \right)$, a correction factor of up to 1.5% should be taken into account.

* sudrescu@mit.edu
† rgarciar@mit.edu
‡ robert.berger@uni-marburg.de

[1] DIRAC, a relativistic ab initio electronic structure program, Release DIRAC19 (2019), written by A. S. P. Gomes, T. Saue, L. Visscher, H. J. Aa. Jensen, and R. Bast, with contributions from I. A. Aucar, V. Bakken, K. G. Dyall, S. Dubillard, U. Ekström, E. Eliav, T. Enevoldsen, E. Faßhauer, T. Fleig, O. Fossgaard, L. Halbert, E. D. Hedegård, B. Heimlich–Paris, T. Helgaker, J. Henriksson, M. Iliaš, Ch. R. Jacob, S. Knecht, S. Komorovský, O. Kullie, J. K. Lærdahl, C. V. Larsen, Y. S. Lee, H. S. Nataraj, M. K. Nayak, P. Norman, G. Olejniczak, J. Olsen, J. M. H. Olsen, Y. C. Park, J. K. Pedersen, M. Pernpointner, R. di Remigio, K. Ruud, P. Sałek, B. Schimmelpfennig, B. Senjean, A. Shee, J. Sikkema, A. J. Thorvaldsen, J. Thyssen, J. van Stralen, M. L. Vidal, S. Villaume, O. Visser, T. Winther, and S. Yamamoto (available at `http://dx.doi.org/10.5281/zenodo.3572669`, see also `http://www.diracprogram.org`).

[2] L. Visscher and K. G. Dyall, "Dirac-fock atomic electronic structure calculations using different nuclear charge distributions," At. Data Nucl. Data Tables **67**, 207–224 (1997).

[3] L. W. Wansbeek, S. Schlesser, B. K. Sahoo, A. E. L. Dieperink, C. J. G. Onderwater, and R. G. E. Timmermans, "Charge radii of radium isotopes," Phys. Rev. C **86**, 015503 (2012).

[4] KM Lynch, SG Wilkins, J Billowes, CL Binnersley, ML Bissell, K Chrysalidis, Thomas Elias Cocolios, T Day Goodacre, RP de Groote, Gregory James Farooq-Smith, *et al.*, "Laser-spectroscopy studies of the nuclear structure of neutron-rich radium," Phys. Rev. C **97**, 024309 (2018).

[5] R. Meyer, "Trigonometric interpolation method for one-dimensional quantum-mechanical problems," J. Chem. Phys. **52**, 2053–2059 (1970), https://doi.org/10.1063/1.1673259.

[6] TA Isaev and R Berger, "Lasercooled radium monofluoride: A molecular all-in-one probe for new physics," arXiv preprint arXiv:1302.5682 (2013).

[7] JL Dunham, "The energy levels of a rotating vibrator," Phys. Rev. **41**, 721 (1932).

[8] Stefan Knecht and Trond Saue, "Nuclear size effects in rotational spectra: A tale with a twist," Chem. Phys. **401**, 103–112 (2012).

[9] Adel Almoukhalalati, Avijit Shee, and Trond Saue, "Nuclear size effects in vibrational spectra," Phys. Chem. Chem. Phys. **18**, 15406–15417 (2016).

[10] AHM Ross, RS Eng, and H Kildal, "Heterodyne measurements of $^{12}C^{18}O$, $^{13}C^{16}O$, and $^{13}C^{18}O$ laser frequencies; mass dependence of Dunham coefficients," Opti. Comm. **12**, 433–438 (1974).

[11] Harold Jeffreys, "On certain approximate solutions of lineae differential equations of the second order," Proceedings of the London Mathematical Society **2**, 428–436 (1925).

[12] Gregor Wentzel, "Eine Verallgemeinerung der Quantenbedingungen für die Zwecke der Wellenmechanik," Z. Phys. **38**, 518–529 (1926).

[13] Hendrik Anthony Kramers, "Wellenmechanik und hal-

bzahlige Quantisierung," Z. Phys. **39**, 828–840 (1926).
[14] Leon Brillouin, "The wave mechanics of schrödinger; a general method of solution by successive approximations," Account Give back. Weekly. Seances Acad. Sci. **183**, 24–26 (1926).
[15] Ph R Bunker, "The nuclear mass dependence of the dunham coefficients and the breakdown of the born-oppenheimer approximation," J. Mol. Spectrosc. **68**, 367–371 (1977).
[16] James KG Watson, "The isotope dependence of diatomic dunham coefficients," J. Mol. Spectrosc. **80**, 411–421 (1980).
[17] Robert J Le Roy, "Improved parameterization for combined isotopomer analysis of diatomic spectra and its application to hf and df," J. Mol. Spectrosc. **194**, 189–196 (1999).
[18] H Knöckel and E Tiemann, "Isotopic field shift in the transition $A0^+ - X^1\Sigma^+$ of PbS," Chem. Phys. **68**, 13–19 (1982).
[19] J Schlembach and E Tiemann, "Isotopic field shift of the rotational energy of the pb-chalcogenides and tl-halides," Chem. Phys. **68**, 21–28 (1982).
[20] RF Garcia Ruiz, R Berger, J Billowes, CL Binnersley, ML Bissell, AA Breier, AJ Brinson, K Chrysalidis, T Cocolios, B Cooper, *et al.*, "Spectroscopy of short-lived radioactive molecules," Nature **581**, 396 (2020).
